# Supplementary material for: Techniques for Constructing Efficient Lock-free Data Structures
Source: arXiv:1712.05406 source file (2017-12-14)
Supplement: Supplementary file 1 [file appendix-hybridnorec.tex]

In order to understand how data structures implemented with hybrid TM would perform, relative to our accelerated template implementations, we implemented the unbalanced BST using Hybrid NOrec, which is arguably the fastest hybrid TM implementation with publicly available code.
We used the same implementation of Hybrid NOrec that was used by Brown and Ravi in~\cite{browncost}.
This is an optimized version that follows the approach in~\cite{hynorecriegel}.
We implemented the BST using Hybrid NOrec by wrapping sequential code for the BST operations in transactions, and replacing each read from (resp., write to) shared memory with a read (resp., write) operation provided by Hybrid NOrec.

In practice, to use a hybrid transactional memory algorithm, one links a compiled hybrid transactional memory library to their code, and then makes a \textit{function call for each read and write} to shared memory.
This can cause enormous overhead.
To avoid this overhead, we compiled this implementation of Hybrid NOrec \textit{directly} into the code for the BST.
Consequently, the Hybrid NOrec functions for reading and writing from shared memory are inlined in our BST code, and are optimized out by the compiler, so no such function calls are actually made.
This is highly favourable to Hybrid NOrec (and likely unrealistic). %, since, in practice, one uses a hybrid transactional memory \textit{library}, which %a compiled library implementation of Hybrid NOrec would 
%involves performing a \textit{function call for each read and write} to shared memory in the unbalanced BST algorithm, which would incur significant overhead.

\begin{fullver}
\begin{figure}[tb]
\begin{minipage}{\textwidth}
\centering
    \setlength\tabcolsep{0pt}
    \hspace{-0.05\textwidth}
    \begin{tabular}{m{0.03\textwidth}m{0.666\textwidth}}
        &
        \fcolorbox{black!80}{black!40}{\parbox{\dimexpr 0.666\textwidth-2\fboxsep-2\fboxrule}{\centering\textbf{2x 24-thread Intel E7-4830 v3}}}
        \\
        &
        \fcolorbox{black!50}{black!20}{\parbox{\dimexpr \linewidth-2\fboxsep-2\fboxrule}{\centering {Unbalanced BST (LLX/SCX)\\ Updates w/key range $[0,10^4)$}}}
        \\
        \vspace{-3mm}\rotatebox{90}{{\textbf{Light} workload}} &
        \includegraphics[width=\linewidth]{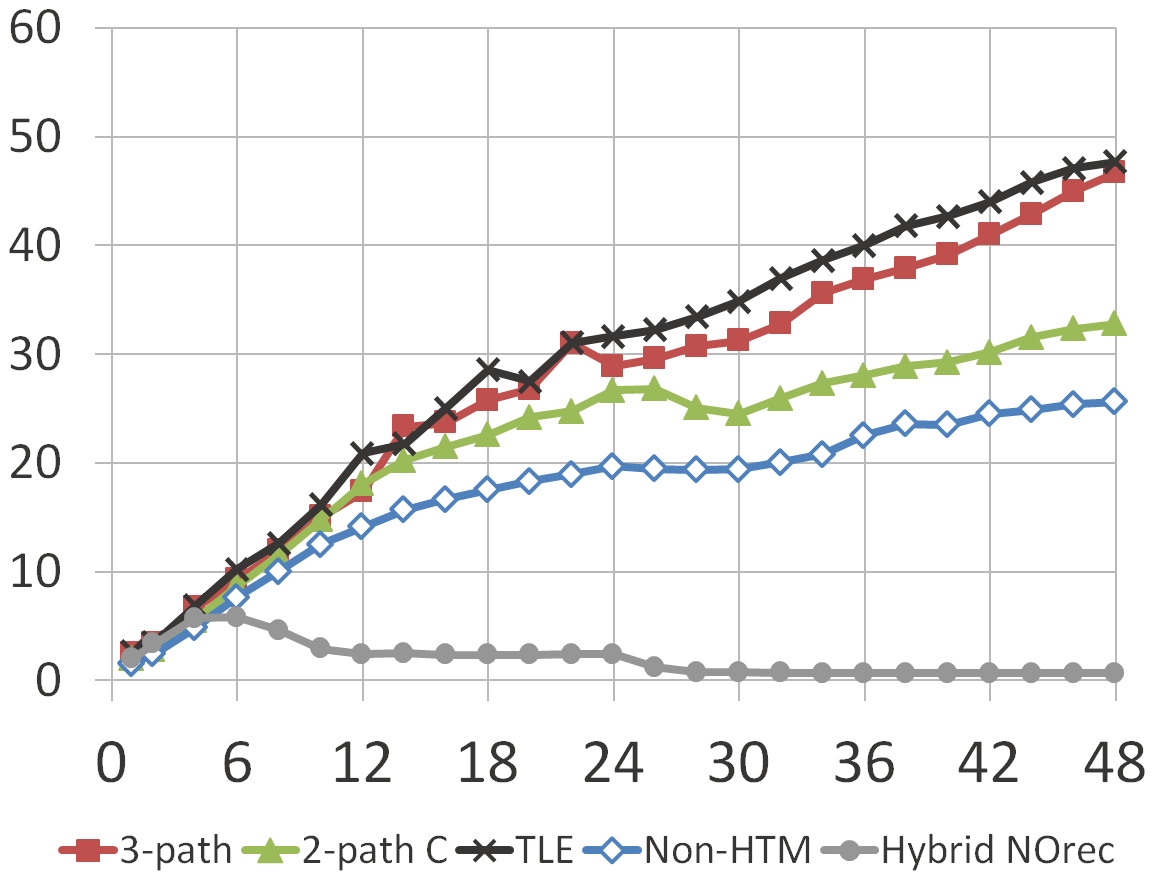}
        \\
    \end{tabular}
    \vspace{-2mm}
    \caption{Results showing throughput (operations per second) versus the number of concurrent processes for an unbalanced BST implemented with different tree update template algorithms, and with the hybrid TM algorithm \textit{Hybrid NOrec}.}
    \label{fig-graphs-hybridnorec}
    \vspace{-3mm}
\end{minipage}
\end{figure}
\end{fullver}

\begin{shortver}
The following graph
\end{shortver}
\begin{fullver}
Figure~\ref{fig-graphs-hybridnorec}
\end{fullver}
compares the performance of the resulting implementation to the other BST implementations discussed in Section~\ref{sec-3path-exp}.
%The workload in Figure~\ref{fig-graphs-hybridnorec} is 
It depicts a light workload, where processes perform 50\% insertions and 50\% deletions on keys drawn uniformly from $[0, 10^4)$.
The x-axis shows the number of concurrent processes.
The y-axis shows completed operations per microsecond.

\begin{shortver}
\medskip

%\begin{figure}[th!]
\begin{minipage}{\textwidth}
\centering
    \setlength\tabcolsep{0pt}
    \hspace{-0.1\textwidth}
    \begin{tabular}{m{0.03\textwidth}m{0.666\textwidth}}%m{0.25\textwidth}}%m{0.24\textwidth}}
        &
%        \multicolumn{2}{c}{%4}{c}{
            %\dimexpr \textwidth-2\fboxsep-2\fboxrule
            \fcolorbox{black!80}{black!40}{\parbox{\dimexpr 0.666\textwidth-2\fboxsep-2\fboxrule}{\centering\textbf{2x 24-thread Intel E7-4830 v3}}}
%        }
        \\
        &
        \fcolorbox{black!50}{black!20}{\parbox{\dimexpr \linewidth-2\fboxsep-2\fboxrule}{\centering {Unbalanced BST (LLX/SCX)\\ Updates w/key range $[0,10^4)$}}} %&
%        \fcolorbox{black!50}{black!20}{\parbox{\dimexpr \linewidth-2\fboxsep-2\fboxrule}{\centering {\footnotesize (a, b)-tree (LLX/SCX)\\ Updates w/key range $[0,10^6)$}}}
        \\
        \vspace{-3mm}\rotatebox{90}{{\textbf{Light} workload}} &
        \includegraphics[width=\linewidth]{chap-3path/figures/perfgraphs/hybridnorec-light-bst10k} %&
        \\
    \end{tabular}
%    \vspace{-2mm}
%    \caption{Results showing throughput (operations per second) versus the number of concurrent processes for an unbalanced BST implemented with different tree update template algorithms, and with the hybrid TM algorithm \textit{Hybrid NOrec}.}
%    \label{fig-graphs-hybridnorec}
%    \vspace{-3mm}
\end{minipage}
%\end{figure}

\medskip
\end{shortver}

The BST implemented with Hybrid NOrec performs relatively well with up to six processes.
However, beyond six processes, it experiences severe negative scaling.
This occurs because Hybrid NOrec increments a global counter in each transaction that writes to shared memory.
This global contention hotspot causes many transactions to abort, simply because they contend on the global counter (and not because they conflict on any data in the tree).
Clearly, the BST implemented with Hybrid NOrec is not a serious competitor for our accelerated implementations.
